# Supplementary material for: SCL(FOL) Revisited
Source: arXiv:2302.05954 source file (2024-03-19)
Supplement: Supplementary file 1 [file appendix.tex]

\section{Exponential Propagation in Weakly-Regular SCL Runs} \label{app:weakly-regular-blowup}

In the original work on SCL \cite{FioriWeidenbach19}, weakly-regular runs have been defined. In such runs, unit propagation is treated differently and is not required to be exhaustive. However, all non-unit propagations still need to be applied before any decision can be made. In the following, we present an example that still requires unnecessary exponential trail growth in weakly-regular runs.

Consider the following clause set:
\begin{align*}
    N = \left\{
\begin{array}{c}
    \begin{array}[]{lclclcl}
        &P & \lor &Q & \lor &S, \\
        &P & \lor &Q & \lor &\neg S, \\
        &P & \lor &\neg Q & \lor &S, \\
        &P & \lor &\neg Q & \lor &\neg S, \\
        &\neg P & \lor &Q & \lor &S, \\
        &\neg P & \lor &Q & \lor &\neg S, \\
        &\neg P & \lor &\neg Q & \lor &S, \\
        &\neg P & \lor &\neg Q & \lor &\neg S,
    \end{array} \\
    \begin{array}{lccl}
        & P & \lor & R(x_1,\ldots,x_n,a,b), \\
        & S & \lor & R(x_1,\ldots,x_n,a,b), \\
        & Q & \lor & R(x_1,\ldots,x_n,a,b), \\
        & \neg P & \lor & R(x_1,\ldots,x_n,a,b), \\
        & \neg Q & \lor & R(x_1,\ldots,x_n,a,b), \\
        & \neg S & \lor & R(x_1,\ldots,x_n,a,b)
    \end{array}
\end{array}
    \right\}
    \end{align*}
    Note that $N$ is unsatisfiable and can be refuted by using only the first eight clauses. Hence, no information about $R$ is needed at all to refute this clause set.
    Furthermore, note that no unit propagation is possible directly from $N'$. Hence, the model building process must start with any decision on $P, Q, S$ or on any ground instance of $R$.

    Consider the case that any of $P, Q, S$ are decided. Then, it becomes mandatory to propagate all $2^n$ ground instances of $R$ by one of the last six clauses before deciding any further literal. In particular, note that it is impossible to refute the clause set by the first eight clauses without a further decision. Hence, to refute the overall clause set, it is necessary to propagate all ground instances of $R$, which are, however, not needed in the actual refutation.

    Next, consider the case that a negated ground instance of $R$ is decided. Then, it is possible and necessary to propagate from the last six clauses. However, this will eventually lead to a conflict. This conflict will be resolved and a new unit clause $R(x_1,\ldots,x_n,a,b)$ will be added. Note that in a weakly-regular run, propagation from this unit clause is not mandatory. However, after the learning of this clause, no negated ground instance of $R$ can be decided anymore.

    Consider the case that a positive ground instance of $R$ is decided. This does not contribute anything to the proof. Either all ground instances are decided at some point, or a decision of $P, Q, S$ happens. In both cases, the trail grew by an exponential number of steps.

    Overall, all weakly-regular runs need to add all $2^n$ different ground instances of $R$ to the trail before being able to refute the clause set with the first eight clauses.

\clearpage

\section{Non-Termination with Bounding Sets} \label{app:non-termination-bounding-set}

\renewcommand{\mrulename}[1]{\ensuremath{}\Rightarrow_{\text{SCL}}^{\text{#1}}}

In \cite{BrombergerEtAl2020arxiv}, a bounding measure for SCL has been introduced. This measure consists of a single set $B$ containing constants that are allowed for instantiation. Hence, all variables in a clause may only be instantiated with a constant from $B$.

For example, consider the bounding set $B = \{a, f(a)\}$. Then, a clause $R(x, f(y))$ can be instantiated in the following ways:
\begin{align*}
    R(a, f(a)), \hspace*{1em} R(f(a), f(a)), \hspace*{1em} R(a, f(f(a))), \hspace*{1em} R(f(a), f(f(a)))
\end{align*}
For a fixed, finite set $N$ of clauses, this bounds the number of considered ground instances to a finite number as well. However, this measure alone does not guarantee termination of SCL. The key aspect is that SCL is able to learn new clauses, which can be instantiated as well. In the following example, we show a regular SCL run that
\\ \noindent (i) only instantiates all clauses with constants from a fixed bounding set $B$,
\\ \noindent (ii) learns infinitely many clauses.

\medskip \noindent
Consider the following input clause set $N$, together with a bounding set $B$:

\vspace*{-1.5em}
\begin{align*}
    N &= \{\neg P(x) \lor \neg P(f(x)), P(x) \lor P(f(x)) \} \\
    B &= \{ a, f(a) \}
\end{align*}
\vspace*{-1.5em}

\noindent Possible instantiations of literals from $N$ are
\begin{align*}
    & P(a), && P(f(a)), && P(f(f(a))), \\
    & \neg P(a), && \neg P(f(a)), && \neg P(f(f(a)))
\end{align*}
Note that $P(f(f(a)))$ is part of this set since $P(f(x))$ is a part of a clause in $N$. In particular, we are allowed to decide on all literals in the above set.

Now, we can construct an example SCL run as follows:

\[
 \begin{array}[]{ll}
 & (\varepsilon; N; \emptyset; 0; \top) \\
 \mrulename{Decide}     & (P(a)^1; N; \emptyset; 1; \top) \\
 \mrulename{Decide}     & (P(a)^1, \neg P(f(f(a)))^2; N; \emptyset; 2; \top) \\
 \mrulename{Propagate}  & (P(a)^1, \neg P(f(f(a)))^2, \neg P(f(a))^{\neg P(x) \lor \neg P(f(x)) \cdot \{x \mapsto a\}}; N; \emptyset; 2; \top) \\
 \mrulename{Conflict}  & (P(a)^1, \neg P(f(f(a)))^2, \neg P(f(a))^{\neg P(x) \lor \neg P(f(x)) \cdot \{x \mapsto a\}}; N; \emptyset; 2; \\ & P(x) \lor P(f(x)) \cdot \{x \mapsto f(a)\}) \\
 \mrulename{Resolve}  & (P(a)^1, \neg P(f(f(a)))^2; N; \emptyset; 2; \\  & \neg P(x) \lor P(f(f(x))) \cdot \{x \mapsto f(a)\}) \\
 \mrulename{Backtrack}  & (P(a)^1; N; \{ \neg P(x) \lor P(f(f(x))) \}; 1; \top)
\end{array}
\]

The illustrated regular SCL run has learned the clause $\neg P(x) \lor P(f(f(x)))$, which is \emph{larger} than any of the original clauses from the input set. Since SCL treats clauses from $N$ and $U$ equivalently, this means that in the next steps, the following instantiations would be valid:
\begin{align*}
     & P(a), && P(f(a)), && P(f(f(a))), && P(f^3(a)), \\
    & \neg P(a), && \neg P(f(a)), && \neg P(f(f(a))), && \neg P(f^3(a))
\end{align*}

\noindent With these instantiations, it is possible to derive clauses containing $f^4$. This process, hence, continues iteratively. Thus, termination is not guaranteed, which motivates the use of our different bounding measure, see Section \ref{subsec:intro:our_contributions:bounding}.
%Clearly, from this clause set, the clause $\neg P(x) \lor P(f(f(x)))$ follows. In SCL, depending on the decisions, this clause could be learned even when only considering instantiations with constants from $B$. For example,  $\neg P(x) \lor \neg P(f(x)) \{x \mapsto a\}$ resolved with $P(x) \lor P(f(x))\{x \mapsto f(a)\}$ yields $\neg P(x) \lor P(f(f(x)))$. This process can be iterated to learn larger clauses. When instantiating such larger clauses, again, with constants from $B$, the clauses grow further. Hence, this restriction alone is not sufficient to guarantee termination.

%\TODO{work out example}
